# Supplementary material for: What does CLIP know about a red circle? Visual prompt engineering for VLMs
Source: arXiv:2304.06712 source file (2023-08-18)
Supplement: Supplementary file 1 [file supp.tex]

\documentclass[10pt,twocolumn,letterpaper]{article}
\usepackage{templatepackage}
\usepackage{times}
\usepackage[dvipsnames]{xcolor}
\usepackage{adjustbox} %
\usepackage{amsfonts}
\usepackage{amsmath}
\usepackage{amssymb}
\usepackage{array}
\usepackage{arydshln}
\usepackage{bbm}
\usepackage[numbers,sort&compress]{natbib}
\usepackage{booktabs}
\usepackage{comment}
\usepackage{dblfloatfix}
\usepackage{dsfont}
\usepackage{float}
\usepackage{graphicx,wrapfig,lipsum}
\usepackage{mathtools,nccmath}
\usepackage{multirow}
\usepackage{pifont}
\usepackage{relsize}
\usepackage{url}
\usepackage{subcaption}

\usepackage[pagebackref=true,breaklinks=true,colorlinks,bookmarks=false]{hyperref}
\usepackage[capitalize]{cleveref}

\makeatletter
\renewcommand{\paragraph}{%
  \@startsection{paragraph}{4}%
  {\z@}{0.25em}{-1em}%
  {\normalfont\normalsize\bfseries}%
}
\makeatother

\makeatletter
\DeclareRobustCommand\onedot{\futurelet\@let@token\@onedot}
\def\@onedot{\ifx\@let@token.\else.\null\fi\xspace}

\newlength{\fHeight}
\setlength{\fHeight}{2ex}

\hfuzz=5.002pt
\hbadness=10000

\templatepackagefinalcopy

\iftemplatepackagefinal\pagestyle{empty}\fi

\begin{document}

\begin{center}
	\textbf{\Large Appendix}
\end{center}
\input{06-supplementary.tex}

{\small\bibliographystyle{ieee_fullname}
\bibliography{refs}}

\end{document}
